# Supplementary material for: CatVersion: Concatenating Embeddings for Diffusion-Based Text-to-Image Personalization
Source: arXiv:2311.14631 source file (2023-11-30)
Supplement: Supplementary file 1 [file supp_beginning.tex]

\clearpage
\setcounter{page}{1}
\maketitlesupplementary

% \section{Rationale}
% \label{sec:rationale}
% % 
% Having the supplementary compiled together with the main paper means that:
% % 
% \begin{itemize}
% \item The supplementary can back-reference sections of the main paper, for example, we can refer to \cref{sec:intro};
% \item The main paper can forward reference sub-sections within the supplementary explicitly (e.g. referring to a particular experiment); 
% \item When submitted to arXiv, the supplementary will already included at the end of the paper.
% \end{itemize}
% % 
% To split the supplementary pages from the main paper, you can use \href{https://support.apple.com/en-ca/guide/preview/prvw11793/mac#:~:text=Delete%20a%20page%20from%20a,or%20choose%20Edit%20%3E%20Delete).}{Preview (on macOS)}, \href{https://www.adobe.com/acrobat/how-to/delete-pages-from-pdf.html#:~:text=Choose%20%E2%80%9CTools%E2%80%9D%20%3E%20%E2%80%9COrganize,or%20pages%20from%20the%20file.}{Adobe Acrobat} (on all OSs), as well as \href{https://superuser.com/questions/517986/is-it-possible-to-delete-some-pages-of-a-pdf-document}{command line tools}.

\section{Further Analysis of the CLIP Feature-Dense Space}
\label{sec:supp_invspace}
To search for the feature-dense space of the CLIP text encoder, we analyze the importance of different layers of the CLIP text encoder in concept learning. Specifically, inspired by Kumari et al. \cite{kumari2023multi}, we fine-tune the CLIP text encoder of Stable Diffusion to align target concepts with the given text. For instance, given input text "cat statue", we utilize several images containing the personalized cat statue to fine-tune the CLIP text encoder in Stable Diffusion. We use the change in the parameters of each layer of the CLIP text encoder to indicate their importance in personalized concept learning, and the formula for calculating the parameter variations is as follows:
\begin{equation}
\Delta_l=\frac{\left\|\theta_l^{\prime}-\theta_l\right\|}{\left\|\theta_l\right\|}
\end{equation}
where $\theta_l$ represents the pre-trained parameter values, and $\theta_l^{\prime}$ represents the fine-tuned parameter values.
We calculate the average parameter variations for each two layers of the CLIP text encoder and visualize these variations. As shown in Figure \ref{fig:supp_param_change}, as the layers of the CLIP text encoder deepen, the average change in parameters increases. This means that the deep level of CLIP text encoders is more important for personalized concept learning.

In addition, we optimize the concatenated residual embeddings of every two layers in the CLIP text encoder to explore the most effective feature space for personalized concept inversion. These embeddings learn the gap between the personalized concept and its base class by adjusting weights in self-attention calculations. Subsequently, we perform experiments on diverse datasets and visualize the resulting generated outputs. Visualizing the generated results obtained from inversion in different layers of the CLIP text encoder can clarify the impact of each self-attention layer on diffusion-based text-to-image generation.
As shown in Figure~\ref{fig:supp_invspace}, optimizing residual embeddings at different layers of the CLIP text encoder has different effects on personalized generation results. Specifically, in the early layers, optimizing embeddings to learn personalized concepts combined with free text for guiding generation tends to generate images containing simple and concrete concepts in the prompt. As optimization progresses from shallow to deep layers, the outputs are more enriched, incorporating not only concrete concepts but also integrating more abstract and complex concepts. This indicates that different layers of the CLIP text encoder have varying levels of integration for the words in the input text. Shallow layers exhibit less integration, while deeper layers show more integration. More integration corresponds to more abstract feature representations. Therefore, we position the feature-dense space of the CLIP text encoder in the final few layers. 
\begin{figure}[t]
  \centering
   \includegraphics[width=1\linewidth]{figures/supp_param_change.pdf}
   \vspace{-20pt}
   \caption{\textbf{Visualization of Parameter Variations}. We visualize the average change in weights for each two layers of the CLIP text encoder. 
   }
   \label{fig:supp_param_change}
\end{figure}

\begin{table}[t]
\centering
\resizebox{\columnwidth}{!}{
  \begin{tabular}{lccc}
    \toprule
    Method & Text Alignment$ \uparrow$  & Image Alignment$ \uparrow$  & Overall $\uparrow$ \\ 
    \midrule
    All Layers & 0.1735 & \textbf{0.8345} & 0.3805 \\ 
    Shallow & 0.1564 & 0.8306 & 0.3604 \\ 
    Intermediate & 0.2471 & 0.6328 & 0.3954 \\ 
    \textbf{Deep} & \textbf{0.2852} & 0.7891 & \textbf{0.4744} \\
    
    \bottomrule
  \end{tabular}
}
\vspace{-0.5em}
\caption{\textbf{Ablation Study}. We conducted ablation experiments on selecting different layers of CLIP text encoders for inversion. Verified the rationality of feature-dense space selection.}
\label{tab:supp_ablation}
\end{table}

\begin{figure*}[t]
  \centering
   \includegraphics[width=1\textwidth]{figures/supp_invspace.pdf}
    % \vspace{-15pt}
   \caption{\textbf{Additional Results for Multi-layer Inversion Visualization}. The results indicate that the self-attention layers of different depths focus on integrating different information. Moreover, the focus of information integration shifts from concreteness to abstraction.
   }
   \label{fig:supp_invspace}
\end{figure*}

\section{The Significance of Modifying Evaluation Metric}
\label{sec:supp_metric}
Since we measure the similarity between paired CLIP images of text-guided generated images,
the CLIP image alignment score do not adapt well in evaluating personalized generation. It measures the similarity of all image features, which is susceptible to difference between the non-object parts of the reference image and the generated image. For example, the CLIP image alignment score calculated by the method of generating images that are easily overfitted to the training scene will be very high, but the majority of the reasons are attributed to overfitting of the background.

To bridge this gap, We obtain the mask of the personalized concept in both the generated and reference images. Subsequently, we calculate the CLIP image alignment score for the region within the mask. This is conducive to focusing attention on the reconstruction of personalized concepts, without being affected by non-object parts.

\section{Detailed Quantitative Setting}
\label{sec:supp_quantitative}
We compare CatVersion with four state-of-the-art methods and conduct quantitative research using paired CLIP alignment scores. Specifically, we measure paired CLIP alignment scores based on 12 datasets from existing methods \cite{gal2022image,ruiz2023dreambooth,tewel2023key}. To achieve unbiased evaluation on editability, we guide image generation using different texts based on four editing categories: attribute transfer, scene transformation, action editing, and concept addition, and then calculate the average CLIP text-to-image alignment score. We improve the CLIP image-to-image alignment score, as mentioned in Section \ref{sec: metric}. And we calculate the CLIP image-to-image alignment score between the generated image and the reference image. Please note that for each method, we fix the seed to generate 100 images for the paired CLIP alignment scores calculation, respectively.

\begin{figure*}[t]
  \centering
   \includegraphics[width=1\textwidth]{figures/supp_our_result1.pdf}
    % \vspace{-15pt}
   \caption{\textbf{Additional Results of Our Method}. Our CatVersion achieves a better balance between faithful reconstruction of the target concept and more robust editability.
   }
   \label{fig:supp_our_result1}
\end{figure*}

\section{Additional Ablation Study}
\label{sec:supp_ablation}
We ablate the feature-dense space and verify the effectiveness of inversion in this space. We use the setup of Section~\ref{sec: clip_space} and divide the inversion space of the CLIP text encoder into shallow, intermediate, deep, and all layers to compute the paired CLIP cosine alignment scores. We measure the balanced performance in the form of the product of CLIP image and text cosine alignment scores.

As shown in Table~\ref{tab:supp_ablation}, inversion in all layers demonstrates the highest CLIP image alignment score, but its CLIP text alignment score is low due to overfitting the scene of the training image. Comparatively, the inversion on the deep layer, i.e., the feature-dense space we utilize, achieves the highest CLIP text alignment scores with the best overall personalized effect. 
In addition, we find that the CLIP text alignment scores show a significant trend of increasing as the number of layers selected for inversion deepens, which also demonstrates the integration of the CLIP text encoder.

% our result 
% \begin{figure*}[t]
%   \centering
%    \includegraphics[width=1\textwidth]{figures/supp_our_result1.pdf}
%     % \vspace{-15pt}
%    \caption{\textbf{Additional Results of Our Method}. Our CatVersion achieves a better balance between faithful reconstruction of the target concept and more robust editability.
%    }
%    \label{fig:supp_our_result1}
% \end{figure*}

\begin{figure*}[t]
  \centering
   \includegraphics[width=1\textwidth]{figures/supp_our_result2.pdf}
    % \vspace{-15pt}
   \caption{\textbf{Additional Results of Our Method}. Our CatVersion achieves a better balance between faithful reconstruction of the target concept and more robust editability.
   }
   \label{fig:supp_our_result2}
\end{figure*}

\begin{figure*}[t]
  \centering
   \includegraphics[width=1\textwidth]{figures/supp_our_result3.pdf}
    % \vspace{-15pt}
   \caption{\textbf{Additional Results of Our Method}. Our CatVersion achieves a better balance between faithful reconstruction of the target concept and more robust editability.
   }
   \label{fig:supp_our_result3}
\end{figure*}

\begin{figure*}[t]
  \centering
   \includegraphics[width=1\textwidth]{figures/supp_our_result4.pdf}
    % \vspace{-15pt}
   \caption{\textbf{Additional Results of Our Method}. Our CatVersion achieves a better balance between faithful reconstruction of the target concept and more robust editability.
   }
   \label{fig:supp_our_result4}
\end{figure*}

\begin{figure*}[t]
  \centering
   \includegraphics[width=1\textwidth]{figures/supp_our_result5.pdf}
    % \vspace{-15pt}
   \caption{\textbf{Additional Results of Our Method}. Our CatVersion achieves a better balance between faithful reconstruction of the target concept and more robust editability.
   }
   \label{fig:supp_our_result5}
\end{figure*}

% comparison
\begin{figure*}[t]
  \centering
   \includegraphics[width=1\textwidth]{figures/supp_compare.pdf}
    % \vspace{-15pt}
   \caption{\textbf{Additional Comparisons with Existing Methods}. Our CatVersion more faithfully restores personalized concepts and achieves more powerful editing capabilities in the combination of various concepts and free text.
   }
   \label{fig:supp_compare1}
\end{figure*}
